# Supplementary material for: StreamRL: Scalable, Heterogeneous, and Elastic RL for LLMs with Disaggregated Stream Generation
Source: arXiv:2504.15930 source file (2025-04-22)
Supplement: Supplementary file 1 [file appendix.tex]

\section{Appendix}
\label{sec:appendix}
